# Supplementary material for: Machine Learning-based Low Overhead Congestion Control Algorithm for Industrial NoCs
Source: arXiv:2302.12779 source file (2023-02-24)
Supplement: Supplementary file 1 [file appendix.tex]

\section*{Appendix A}

\begin{table}[h]
\begin{tabular}{l|l}
\hline
Event         & Symbol        \\ \hline
$p(A \cap B)$ & $\lambda_d^i$ \\ \hline
$p(A)$        & $p_\sigma^i$  \\ \hline
$p(B)$        & $\lambda_l^i$ \\ \hline
$p(A|B)$      & $p_d$      \\ \hline   
\end{tabular}
\end{table}

\begin{flalign}
    & p(A \cap B)  \leq p(A) \\
    \implies & p(A|B)p(B) \leq p(A) \\
    \implies & p(A|B) \Big( \frac{\lambda_\sigma^i}{1-p(A|B)} \Big) \leq p(A) \\
    \implies & p(A|B) \leq \frac{p(A)}{\lambda_\sigma^i + p(A)}
\end{flalign}
